# Supplementary material for: Population based change-point detection for the identification of homozygosity islands
Source: arXiv:2111.10187 source file (2021-11-19)
Supplement: Supplementary file 1 [file Appendix_A_consistency.tex]

\section{Proof of consistency}
\label{appendix: proof_of_consistency}
\subsection{Penalized likelihood estimator consistency}

    We restate and prove the theorem for the consistency of the PL estimator.

    \begin{theorem}
    Let $\widehat{C}$ be the estimator given by \eqref{hatC}, considering $\lambda$ fixed. Suppose that the family of distributions satisfy conditions (PL-i) and (PL-ii).
    Suppose that $R(C) > R(C')$ holds whenever
    $C\supset C'$. Finally, assume that the function $J(n)$ satisfies $J(n)/v(n) \longrightarrow\infty$ and $J(n)/n \longrightarrow 0$ when $n\rightarrow \infty$. Then, $\widehat{C}=C^*$ eventually almost surely as $n\to\infty$.
    \end{theorem}
    \begin{proof}	
        First we will prove that $\widehat{C}$ will
        almost surely contain $C^*$. Let $C\in\C$ such that 
        $C\not\supseteq C^*$. Then by hypothesis (i) we have that eventually almost surely 
        \[
        \frac1nl(C;\bx) - \frac1nl(C^*;\bx) \;<\; -\frac{\alpha}2 \,.
        \]
        On the other hand, as $J(n)=o(n)$ and $R(C)$ is bounded  we have that
        \[
        \lambda (R(C) - R(C^*)) \frac{J(n)}n \;\to \; 0
        \]
        as $n\to\infty$. Therefore, eventually almost surely we have
        \[
        \pl(C^*;\bx) \;< \; \pl(C;\bx)\,.
        \]
        As the number of $C\not\supseteq C^*$ is finite we have that eventually almost surely $\widehat C\supseteq C^*$. 
        
        Lets prove that $\widehat C \not\supset C^*$. Assume $C\supset C^*$ so that $R(C) > R(C^*)$ and $l^*(C) = l^*(C^*)$. Then, by hypothesis (ii), we have that 
        \begin{equation}
        \begin{split}
            \pl(C^*;\bx) - \pl(C;\bx)\;&\leq\; v(n) + \lambda(R(C^*) - R(C)) J(n)\\
            & <\; 0
        \end{split}
        \end{equation}
        eventually almost surely as $n\to\infty$. As a results we have that $\widehat C=C^*$ eventually almost surely as $n\to\infty$. 
    \end{proof}

\subsection{Hierarchical estimator consistency}
    
    We now state and prove the consistency of the hierarchical estimator.

    \begin{theorem}
        Let $\widehat{C}_{HS}$ be the estimator computed by the hierarchical algorithm, considering $\lambda$ fixed. Suppose that the family of distributions satisfy conditions (H-i), (H-ii) and (H-iii).
        Suppose that $R(C) > R(C')$ holds whenever $C\supset C'$, and that there exists a function $\rho: 1:m \times 1:m \longrightarrow \mathbb{R}$ such that, if $C = \{c_1,\ldots,c_k\}$, then $R(C) = \sum_{j=1}^{k+1} \rho(c_{j-1}+1, c_j)$..    Finally, assume that the function $J(n)$ satisfies $J(n)/v(n) \longrightarrow\infty$ and $J(n)/n \longrightarrow 0$ when $n\rightarrow \infty$. Then, $\widehat{C}_{HS} = C^*$ eventually almost surely as $n\to\infty$.
    \end{theorem}
	
\begin{proof}
    The proof is divided in two parts; first, we show that, at any given possible scenario, the algorithm takes a correct choice almost surely; then, an induction argument will guarantee that the algorithm is consistent.

	\paragraph{Part 1} For every integer interval $I = r:s$ the algorithm receives as an input, we either have
	
	\begin{itemize}
	    \item [(a)] There are no change points in $I$;
	    \item [(b)] There are change points in $I$.
	\end{itemize}
	
	The correct decision for the algorithm in case \textbf{(a)} is to halt, not performing more recursive calls for that interval; for \textbf{(b)}, the correct decision is to choose any of the change points available and perform recursive calls on the sub intervals. 
	
	We assert that the algorithm will take the correct decision almost surely for both cases.
	
	\paragraph{(a)} Suppose $I$ has no change points inside and let $u \, \in\, r:(s-1)$. We have
	
	\begin{align*}
	h(s) - h(u) &= -\left[l(I; \mathbf{x}_I) - l(r:u; \mathbf{x}_I) - l((u+1):s; \mathbf{x}_I)\right] + \\
	& + J(n)\lambda\left[\rho(r, s) - \rho(r, u) -\rho(u+1, s)\right]\\
	& \overset{a.s.}{<} v(n) + J(n)\lambda\left[\rho(r, s) - \rho(r, u) -\rho(u+1, s)\right] \\
	&< 0\quad,
	\end{align*}
	
	eventually almost surely as $n \longrightarrow \infty$, because $\left[\rho(r, s) - \rho(r, u) -\rho(u+1, s)\right] < 0$. Hence, no splitting will be done eventually almost surely, and the algorithm will not perform more recursive calls.

    \paragraph{(b)}   Now we have to prove that the algorithm will almost surely split at change points only. Hypothesis \ref{hyp_strict_max} directly implies that, for any $u$ that is not a change point, there exists a change point $c^*$ in $I$ such that

\begin{equation*}
    h_I^*(u) > h_I^*(c^*) \quad.    
\end{equation*}    

    When considering the loss of not splitting this interval, remember that
    
\begin{equation*}
    l(\emptyset; X_I) \leq l({c}; X_I), \quad \forall \, c \,\in\,r:(s-1)\quad,
\end{equation*}
    
    hence $h_I^*(s) > h_I^*(c^*)$, since $h_I^*(s)$ represents no splitting is performed.
    
    Finally, notice that condition (H-i) and $J(n) \, \in \, O(n)$ implies that guarantees that $\frac{1}{n}h(u) \overset{a.s.}{\longrightarrow} h^*(u)$. Hence,

\begin{equation*}
   \frac{h(u) - h(c^*)}{n} = h^*(u) - h^*(c^*) > 0 \quad,
\end{equation*}    
    
    concluding that
    
\begin{equation*}
   h(u) - h(c^*) \quad,
\end{equation*}    

    eventually almost surely as $n \, \longrightarrow \infty$.
    
    \paragraph{Part 2}  We finish the proof using mathematical induction on the number of variables $m$. 
    
    If $m = 1$, then there is no possibility for change points, and the algorithm will not even have comparisons to make. Hence, the change point set is always empty by construction, and therefore is consistent.
    
    Suppose that the algorithm is consistent for every $\tilde{m} <= m-1$, we will prove that it will be consistent for $m$.
    
    The first run of the algorithm is on the interval $1:m$. By \textbf{Part 1}, if there are no change points, the algorithm will almost surely not split the interval and will halt since no other recursive calls will be made, and hence will be consistent.
    
    If there are change points, take $c_0 = 0$ and $c_{|C^*|+1} = m$.  \textbf{Part 1} tells us again that the algorithm eventually almost surely takes the correct choice and splits at a change point $c$. After the split, recursive calls are made on $1:c$ and on $(c+1):m$. But the length of these arrays are at most $m-1$, and by induction hypothesis we have that the algorithm will eventually almost surely retrieve all the change points in $1:c$ and in $(c+1):m$, obtaining then the whole change point set.
    
\end{proof}

    Hypothesis \ref{hyp_strict_max} is very difficult to prove directly in general. We now state a set of hypothesis that are easier to prove and imply the desired condition.

\begin{theorem}\label{conditions_hyp3_HS}
    Let the change points set in $I$ be  $\{c_0, \ldots, c_k\}$. Assume that 

\begin{enumerate}
    \item[(a)] There exists a point $c\,\in\,I$ such that $h_I^*(s) > h_I^*(c)$. That is, there is at least one point with loss smaller than the loss of not splitting;
    \item[(b)] The function $h_I^*$ is concave between consecutive change points. That is, $h_I^*$ is concave in $[c_j, c_{j+1}]$ for any $j\,\in\,{1, \ldots, k-1}$;
    \item[(c)] If $h_I^*(u)$ is constant in $[c_j, c_{j+1}]$, then it is equals to $h_I^*(s)$. 
\end{enumerate}    
    
    Then, we have

\begin{equation*}
 \min_{c \in (I\setminus\{s\})\cap C^*} \; h_I^*(c)\;<\; \min_{c \not\in (I\setminus\{s\})\cap C^*} \; h_I^*(c) \,. 
\end{equation*}
\end{theorem}

\begin{proof}
    Let $h_I^*(u)$ be the minimum value of $h_I^*$ in $I$. First, notice that $h_I^*(u) \leq h_I^*(c) < h_I^*(s)$, so the minimum is smaller than the loss without splitting. We now prove that $u$ must be a change point.
    
    Suppose, by absurd, that $u$ is not a change point, and let $c_j$ and $c_{j+1}$ be the change points that surround it. Since $h_I^*$ is concave in $[c_j, c_{j+1}]$, if the minimum is attained at an interior point, then $h_I^*$ must be constant. However, by the last hypothesis, it would imply that $h_I^*(u) = h_I^*(s)$, reaching an absurd.
\end{proof}

    We prove that these conditions hold when i.i.d. observations from families of distributions satisfying some properties. These properties are general to hold for several distributions, in particular for the categorical distribution and the normal distribution with known variance.

\subsection*{Conditions for the i.i.d. case}
    
    Assume that the random variables are i.i.d. and write $\ell$ as the log-likelihood of a single random variable. If $\ell$ is continuous and $\frac{1}{n}\ell \overset{a.s.}{\longrightarrow} \ell^*$, then the log-likelihood of the interval $I$ is 
    
\begin{equation*}
    l^*(I) = |I|\ell^*(\theta_{I}) \quad,
\end{equation*}

    where $\theta_{I}$ is the limit of  $\hat{\theta}_I$.

    Assume further that the parametric space $\Theta$ is an open convex subset of  $\mathbb{R}^d$ for some integer $d$, and
    
\begin{enumerate}
    \item[(i)] $\ell^*: \Theta \mapsto \mathbb{R}$ is strictly convex, has second order derivatives $\Theta$;
    \item[(ii)] For every interval $I$, we have that $\theta_I = \sum_{r=1}^{k^*} \frac{|I \cap I_r^*|}{|I|} \theta_r^*$.
    
\end{enumerate}
    
    Under these hypothesis, given $c_j < u < c_{j+1}$, the function $h^*$ can be written as
    
\begin{equation*}
    h_I^*(u) = -(u-r+1)\ell^*(\theta_{r:u}) - (s-u)\ell^*(\theta_{(u+1):s}) \quad.
\end{equation*}

    Defining $t := t(u) = \frac{c_j-r+1}{u-r+1}$, we can write 

\begin{equation*}
    \theta(u) = \theta_{r:u} = t(u)\theta_{r:c_j} + (1-t(u))\theta_{j+1}^* \quad.
\end{equation*}

    We now state the theorem

\begin{theorem}\label{conditions_iid_HS}
    Under the hypothesis stated above, the family of distributions satisfy the hypothesis of theorem \ref{conditions_hyp3_HS}.
\end{theorem}
    
\begin{proof}
    
    We prove each of the condition separately.
    
    \paragraph{Concavity} To prove that $h^*$ will be concave in the interval $[c_j, c_{j+1}]$, it is sufficient to show that  $(u-r+1)\ell^*(\theta_{r:u})$ and $(s-u)\ell^*(\theta_{(u+1):s})$ are convex in this interval.
    
    Let $g(u) := (u-r+1)\ell^*(\theta(u))$, the first derivative is
    
\begin{align*}
    g'(u) 
    &= \ell^*(\theta(u)) + (u-r+1)t'(u)\big\langle \theta_{r:c_j}-\theta_{j+1}^*, \,\nabla \ell^*(\theta(u))\big\rangle\\
    &=  \ell^*(\theta(u)) -t(u)\big\langle \theta_{r:c_j}-\theta_{j+1}^*, \,\nabla \ell^*(\theta(u))\big\rangle \quad ,\\
\end{align*}
    
    where the second equality follows from the fact that $(u-s+1)t'(u) = -t(u)$.
    
   The second derivative is then
    
\begin{align*}
    g''(u) 
    % first term
    &= \overbrace{t'(u)\big\langle \theta_{r:c_j}-\theta_{j+1}^*, \,\nabla \ell^*(\theta(u))\big\rangle - t'(u)\big\langle \theta_{r:c_j}-\theta_{j+1}^*, \,\nabla \ell^*(\theta(u))\big\rangle}^{=0}\\
    % second term
    &+(-t'(u)t(u))\big\langle \theta_{r:c_j}-\theta_{j+1}^*, \, H_{\theta(u)}({\ell^*})(\theta_{r:c_j}-\theta_{j+1}^*)\big\rangle\\
    &\geq 0 \quad.
\end{align*}
    
    The term $H_{\theta(u)}(\ell^*)$ denotes the Hessian matrix of $\ell^*$ evaluated at $\theta(u)$. Since it is positive definite and  $-t'(u)t(u) \geq 0$, the last inequality holds.
    
    The same proof outline can be followed to prove that $(s-u)\ell^*(\theta_{(u+1):s})$.

%%%%%%%%%%%%%%%
    
\paragraph{Plateau at no splits} We show that, if $h_I^*$ is constant in an interval $[c_j, c_{j+1}]$, then the loss must be the same as not splitting. We first prove a very simple proposition.
    
\begin{prop}
    Let $f,g:\mathbb{R}\mapsto\mathbb{R}$ be convex functions and twice differentiable. If there exists a constant $\alpha$ such that

\begin{equation*}
    f(x) + g(x) = \alpha \quad,
\end{equation*}

    then $f$ and $g$ must be linear functions.

\end{prop}    
    
\begin{proof}
    Differentiating both sides twice, we have
    
\begin{equation*}
    f''(x) + g''(x) = 0 \quad.
\end{equation*}
    
    Since $f''(x) \geq 0$ and $g''(x) \geq 0$, then $f''(x) = 0 = g''(x)$ and the result follows.
    
\end{proof}
    
    Now suppose that $h_I^*(u)$ is constant in $[c_j, c_{j+1}]$. Then, for some $\alpha$, we have
    
\begin{equation*}
    -(u-r+1)\ell^*(\theta_{r:u}) - (s-u)\ell^*(\theta_{(u+1):s}) = \alpha \quad.
\end{equation*}
    
    The proposition above implies that $(u-r+1)\ell^*(\theta_{r:u})$ and $(s-u)\ell^*(\theta_{(u+1):s})$ are linear functions, therefore $\ell^*(\theta_{r:u})$ and $\ell^*(\theta_{(u+1):s})$ are constants. 
    
    By differentiating once, we conclude that $\ell^*(\theta_{r:u}) = \ell^*(\theta_{(u+1):s})$. Remember that $\theta_{r:u}$ and $\theta_{(u+1):c_{j+1}^*}$ are convex combinations. Since $\ell^*$ is strictly convex, we have that $\theta_{r:u}$ and $\theta_{(u+1):c_{j+1}}$ are constants, implying $\theta_{r:c_j } = \theta_{j+1}^* = \theta_{(c_j+1):s}$. But  
\begin{equation*}
    \theta_I = \frac{1}{|I|}\left(|c_j - r + 1|\theta_{r:c_j} + |s - c_j|\theta_{(c_j+1):s}\right) = \theta_{r:c_j} = \theta_{(c_j+1):s} \quad,
\end{equation*}
    and therefore $h_I^*(u) = h_I^*(s)$, proving the result.
    
\paragraph{Minimum at the interior} We finish the proof by showing that the minimum is attained at the interior of $I$. 

    Suppose, by absurd, that the minimum is attained at $h_I^*(s)$. Since $h_I^*(s)$ is also a maximum, we have that the loss in the whole interval $I$ is constant. Following the same computations as above, we conclude that $\theta_i^* = \theta_j^*$ for all $i, j \, \in \, \{0, \ldots, k+1\}$, reaching an absurd, because there is at least one change point.

\end{proof}

\subsection*{Time Complexity}

    We now provide the asymptotic time complexity of the hierarchical algorithm. Albeit $m$ is fixed and only $n$ grows, the number of variables $m$ can be very large in some applications, so it is useful to express the complexity in terms of both.

    \begin{prop}
    \label{prop: hier_complexity}
        The HS algorithm will asymptotically perform exactly $2|C| + 1$ recursive calls. Moreover, its complexity will be $O(T(n, m) + m|C|)$, where $T(n, m)$ is the time complexity to compute the sufficient statistics for the family.
    \end{prop}
    
    \begin{proof}
        
        First, we prove that the algorithm will eventually almost surely do exactly $2|C| + 1$ recursive calls by induction on $|C|$. 
        
        Let $|C| = 0$. The first run of the algorithm is always on $1:m$. Since it is asymptotically correct, it halts after the first iteration. Therefore, the number of recursive calls is $1 = |C| + 1$.
        
        Suppose that it holds for $|C| \leq K-1$ for any value of $m$, we prove that it will hold for $|C| = K+1$. At the first call, the algorithm selects a change point $c$ and creates a recursive call on $1:(c-1)$ and on $(c+1):m$. Let $N_l$ be the number of change points on $1:(c-1)$ and $N_r$ be the number of change points on $(c+1):m$, noting that $N_r + N_l = K-1$. Using induction hypothesis, we have that the algorithm does $2N_l + 1$ calls on $1:(c-1)$ and $2N_r + 1$ on $(c+1):m$. Hence, the total of calls is
    
        $$1 + 2N_l + 1 + 2N_r + 1 = 3 + 2(N_l + N_r) = 3 + 2K - 2 = 2K + 1 \quad. $$

        To obtain the final complexity, note that a call in the interval $r:s$ the algorithm does $|s - r + 1| \leq m + 1$ comparisons and memory checks, and therefore has complexity of $O(m|C|))$. However, we need to pre-compute the sufficient statistics in order to evaluate the loss, which has a complexity of $T(n, m)$. 
    
    \end{proof}

    For the families proposed in this work, $T(n, m) = O(nm)$. If the number of change points $|C|$ is constant, then the final complexity will be linear on $m$.

\vskip 0.2in
