# Supplementary material for: Population based change-point detection for the identification of homozygosity islands
Source: arXiv:2111.10187 source file (2021-11-19)
Supplement: Supplementary file 2 [file Appendix_B_distributions.tex]

\section{Checking hypothesis for different models and distributions}

    We will now verify that the hypothesis of the theorem holds for a categorical and normal distributions. 
    
    In all examples, we will use the notation $C^* = \{c_0^*, \ldots, c_{k^*}^*\}$ and $\theta^* = (\theta_1^*, \ldots, \theta_{k^*}^*)$ for the true change point set and parameters. We will denote $C = \{c_0, \ldots, c_{k}\}$ and $\theta$ for an arbitrary change point set and parameter. 
    
    Furthermore, consider $I_j = (c_{j-1}+1):c_j$ and $I_r^* = (c_{r-1}^*+1):c_r^*$ through all examples.

%%%---------------------------------------------%%%
\subsection{Independent with categorical distribution}

Let $A=\{a_1,\dotsc, a_d\}$ be a finite set and let
\[
\F=\{p\in [0,1]^d\colon p(a_i)\geq 0\text{ and } \sum_{i=1}^{d} p(a_i)=1\}
\]
be the family of all  probability distributions over $A$. The likelihood function \eqref{prob} can be written, for $C\in\C$ and $\theta=(p_1,\dots,p_k)$, as 
\begin{equation}
\P_{(C,\theta)}(\bx) = \prod_{j=1}^{k}\prod_{v = c_{j-1}+1}^{c_j} p_j(x_v).
\end{equation}
The log-likelihood for the sample $\{\bx^{(i)}\}_{i=1}^n$, evaluated at the maximum likelihood estimator for $\theta$, can be written as
\begin{equation}
l(C;\bx) = \sum_{j=1}^{k} \sum_{a\in A} N_{I_j}(a) \log \frac{N_{I_j}(a)}{n|I_j|}\,,
\end{equation}
where
\begin{equation}
    N_{I_j}(a) \;=\; \sum_{i=1}^n\sum_{v=c_{j-1}+1}^{c_j}\mathbf{1}\{x^{(i)}_v=a\}
\end{equation}

To check (i) let $C\not\supseteq C^*$. 
%Then there exists an interval $(c_{i-1}+1):c_{i}$, $i\geq 1$,  containing a change point $c^*_j\in C^*$, $1\leq j\leq k-1$. 
By the Law of Large Numbers, we have that 
\[
\frac1n l(C;\bx) \;\to\; \sum_{j=1}^{k}  |I_j| \sum_{a\in A}  \bar p_{I_j}(a) \log \bar p_{I_j}(a) =: l^*(C)\,,
\]
with 
\[
\bar p_{I_j}(a) \;=\; \sum_{r=1}^{k^*}  \frac{|I_j\cap I^*_r|}{|I_j|} p_r^*(a) \qquad a\in A\,. \quad
\]
Moreover we have that 
\begin{equation}
\begin{split}
l^*(C) - l^*(C^*) &\;= \;   \sum_{j=1}^{k} \sum_{r=1}^{k^*} |I_j\cap I^*_r|  \sum_{a\in A}  p_r^*(a) \log \bar p_{I_j}(a)  -  \sum_{r=1}^{k^*} |I^*_r|  \sum_{a\in A}  p_r^*(a) \log p_r^*(a)\\
&=  \; \sum_{j=1}^{k} \sum_{r=1}^{k^*} |I_j\cap I^*_r|  \sum_{a\in A}  p_r^*(a) \log \frac{\bar p_{I_j}(a)}{p_r^*(a)}\\
&< \;0
\end{split}
\end{equation}
unless $\bar p_{I_j} = p_r^*$ for all $r$ and $j$ with $|I_j\cap I^*_r|\neq\emptyset$. But this can only happen if $C\supseteq C^*$, which is a contradiction. 

To verify hypothesis (ii) observe that for any $C\supseteq C^*$
\begin{equation*}
    \begin{split}
    l(C;\bx)  - l(C^*;\bx) \;&=\; \sum_{j=1}^{k} \sum_{a\in A} N_{I_j}(a) \log \frac{N_{I_j}(a)}{n|I_j|} - \sum_{j=1}^{k^*} \sum_{a\in A} N_{I_j^*}(a) \log \frac{N_{I_j^*}(a)}{n|I_j^*|}\\
    &\leq \sum_{j=1}^{k} \sum_{a\in A} N_{I_j}(a) \log \frac{N_{I_j}(a)}{n|I_j|} - \sum_{j=1}^{k^*}  \sum_{a\in A}  N_{I_j^*}(a)  \log p_j^*(a)\,,
    \end{split}
\end{equation*}
where the last inequality follows because $N_{I_j^*}(a)/n|I_j^*|$ are the maximum likelihood estimator for $p_j^*(a)$.  As $C\supseteq C^*$, we have that any interval $I_r^*$ contains one or more intervals $I_j$, and 
\[
N_{I_r^*}(a) \; = \; \sum_{j: I_j\subseteq I_r^*}N_{I_j}(a) \qquad\text{ for all }a\in A\,.
\]
Then, we can write the difference above as
\begin{equation*}
    \begin{split}
\sum_{j=1}^{k} \sum_{a\in A} N_{I_j}(a) \log \frac{N_{I_j}(a)/n|I_j|}{p_{i_j}^*(a)}
    \end{split}
\end{equation*}
where $i_j$ is the corresponding index in $C^*$. Therefore we obtain that 
\begin{equation*}
    \begin{split}
    l(C;\bx)  - l(C^*;\bx) \;&\leq\; \sum_{j=1}^{k}  n |I_j| D(\hat p_j(a) ; p_{i_j}^*(a))\,.
    \end{split}
\end{equation*}
Adapting a well-known inequality (see Lemma 6.3 in \cite{Csiszar2006}) we have that 
\[
D(\hat p_j(a) | p_{i_j}^*(a)) \;\leq\; \sum_{a\in A} \frac{|\hat p_j(a) - p_{i_j}^*(a)|^2}{p_{i_j}^*(a)}\,.
\]
As the difference $N_{I_j}(a) - n|I_j|p_j(a)$ can be written a sum of zero-mean independent random variables with finite variance, we have, by the Law of the Iterated Logarithm (see theorem 3.52 in  \cite{breiman1969probability}) that 
\[
|\hat p_j(a) - p_{i_j}^*(a)| \;\leq\; \sqrt{\frac{c\log\log n|I_j|}{n|I_j|}}
\]
for a given constant $c$, eventually almost surely as $n\to\infty$. Since $|I_j|$ is bounded by $m$, $\log\log n|I_j| = \Theta(\log\log n)$. Hence, there exists $\delta_j > 0$ such that 
\[
|\hat p_j(a) - p_{i_j}(a)| \;\leq\; \sqrt{\frac{\delta_j \log\log n}{n|I_j|}}
\]
eventually almost surely as $n\to\infty$.
Finally, we obtain that 
\begin{equation*}
    \begin{split}
    l(C;\bx)  - l(C^*;\bx) \;&\leq\;  \frac{k\delta_{min}}{p_{\min}} \log\log n\;\leq\; \frac{m\delta_{min}}{p_{\min}}\log\log n \,,
    \end{split}
\end{equation*}
with $p_{\min} = \min\{p_j(a) \colon p_j(a)>0,  j=1,\dots,k^*, a\in A\}$, and $\delta_{min}  = \underset{j \, \in \,\{1,\ldots, k\}}{\min} \delta_j $.  On the other hand, it is ease to see that 
\[
   l(C;\bx)  - l(C^*;\bx) \;\geq\; 0
\]
for any $C\supseteq C^*$. Then, hypothesis (ii) holds for $v(n)=c\log\log n$, for some $c>0$. \\

\subsubsection{Verifying HS conditions}

    To prove that the HS is consistent for the categorical family, we have to prove th conditions for the HS. From the subsection above, we already proved that they hold for condition (H-i) and (H-ii). Only condition (H-iii) is left to prove. However, we only have to show that this family satisfies the conditions for theorem \ref{conditions_iid_HS}.
    
    Assume that no probability parameter is $0$ or $1$. That is, assume that $\Theta$ = $\mbox{int}(\Delta^{d-1})$, with $\Delta^{d-1}$ denoting the simplex in $\mathbb{R}^d$. The previous computation show us that
\begin{equation}
    \frac1n l(C;\bx) \;\to\; \sum_{j=1}^{k}  |I_j| \sum_{a\in A}  \bar p_{I_j}(a) \log \bar p_{I_j}(a) = l^*(C)
\end{equation}

    Since $p\log(p)$ is convex and $C^\infty$ in $(0, 1)$, and $l^*$ is the sum of convex functions, it follows that it is convex and twice differentiable. Moreover, the limit maximum likelihood estimator for an interval $I$ is
    
\[
\bar p_{I_j}(a) \;=\; \sum_{r=1}^{k^*}  \frac{|I_j\cap I^*_r|}{|I_j|} p_r^*(a) \qquad a\in A\,. \quad
\]

    Therefore, all conditions for the theorem holds, and consistency is guaranteed.

%%%---------------------------------------------%%%
\subsection{Independent with normal distribution}

    Consider the family 
    
\begin{equation*}
    \mathcal{F} = \{f_{(\mu,\sigma^2)} \colon (\mu, \sigma^2)\,\in\,\mathbb{R}\times\mathbb{R}_{+} \}
\end{equation*}
    
    where $f_{(\mu, \sigma^2)}$ be the density of a normal distribution with mean $\mu$ and variance $\sigma^2$. We will prove that this family satisfy the conditions of the theorems.
    
     Given $C$ and $\theta = ((\mu_j, \sigma_j^2))_{j=1}^{k}$, the likelihood is given by

\begin{equation*}
    \mathbb{P}_{(C,\theta)}(\mathbf{X}) = \prod_{j=1}^{k}\prod_{c \,\in\, I_j} (2\pi)^{-\frac{n}{2}}(\sigma_j^2)^{-\frac{n}{2}}e^{- \frac{1}{2\sigma_j^2}\sum_{i=1}^n(X_c^{(i)} - \mu_j)^2} \quad.
\end{equation*}
    
    Hence, the log-likelihood is

\begin{equation*}
    l((C,\theta); \mathbf{X}) = \sum_{j=1}^{k}\sum_{c \,\in\, I_j} {-\frac{n}{2}}\log(2\pi) {-\frac{n}{2}}\log(\sigma_j^2) - \frac{1}{2\sigma_j^2}\sum_{i=1}^n(X_c^{(i)} - \mu_j)^2 \quad.
\end{equation*}

    It is straight forward to prove that, conditional to $C$, the maximum likelihood estimator $\hat{\theta}_C$ is given by

\begin{equation*}
     \hat{\theta}_C = ((\hat{\mu}_j, \hat{\sigma}_j^2))_{j=1}^{k} \quad,
\end{equation*}
    
    where 

\begin{align*}
    &\hat{\mu}_j = \frac{1}{n|I_j|} \sum_{c \,\in\, I_j}\sum_{i=1}^n X_c^{(i)} \quad;\\
    &\hat{\sigma}_j^2 = \frac{1}{n|I_j|} \sum_{c \,\in\, I_j}\sum_{i=1}^n (X_c^{(i)} - \hat{\mu}_j)^2 \quad.\\
\end{align*}

The log-likelihood evaluated at $\hat{\theta}_C$ is then

\begin{equation*}
    l(C; \mathbf{X}) = -\frac{nm}{2}(\log(2\pi)+1)-\frac{n}{2}\sum_{j=1}^{k}|I_j|\log(\hat{\sigma}_j^2) \quad.
\end{equation*}

Notice that

\begin{align*}
    \hat{\mu}_j 
    &= \frac{1}{n|I_j|} \sum_{c \,\in\, I_j}\sum_{i=1}^n X_c^{(i)}\\ &= \frac{1}{n|I_j|} \sum_{r=1}^{k^*+1}\sum_{c \,\in\, I_j \cap I_r^*}\sum_{i=1}^n X_c^{(i)}\\
    &= \sum_{r=1}^{k^*}\frac{|I_j \cap I_r^*|}{|I_j|}\left[\frac{1}{n|I_j \cap I_r^*|}\sum_{c \,\in\, I_j \cap I_r^*}\sum_{i=1}^n X_c^{(i)}\right]\\
    &\overset{\mbox{a.s.}}{\longrightarrow} \sum_{r=1}^{k^*}\frac{|I_j \cap I_r^*|}{|I_j|} \mu_r^* =: \mu_j \quad.
\end{align*}

The convergence on the last equations follows due to the Strong Law of Large Numbers. For the variance

\begin{align*}
    \hat{\sigma}_j^2 
    &= \frac{1}{n|I_j|} \sum_{c \,\in\, I_j}\sum_{i=1}^n (X_c^{(i)} -\hat{\mu}_j)^2\\ 
    &= \frac{1}{n|I_j|} \sum_{r=1}^{k^*}\sum_{c \,\in\, I_j \cap I_r^*}\sum_{i=1}^n (X_c^{(i)} - \hat{\mu}_j)^2\\
    &= A_{nj} + B_{nj} + C_{nj} \quad,\\
\end{align*}

where

\begin{align*}
    & A_{nj} =\sum_{r=1}^{k^*}\frac{|I_j \cap I_r^*|}{|I_j|}\left[\frac{1}{n|I_j \cap I_r^*|}\sum_{c \,\in\, I_j \cap I_r^*}\sum_{i=1}^n (X_c^{(i)} - \mu_r^*)^2\right] \quad;\\
    & B_{nj} = -2\sum_{r=1}^{k^*}\frac{|I_j \cap I_r^*|}{|I_j|}(\mu_r^* - \hat{\mu}_j)(\hat{\mu}_{I_j \cap I_r^*}^* - \mu_r^*) \quad; \\
    & C_{nj} = \sum_{r=1}^{k^*}\frac{|I_j \cap I_r^*|}{|I_j|} (\mu_r^* - \hat{\mu}_j)^2 \quad. \\
\end{align*}

    Since they are all continuous functions, we have by the SLLN and continuous mapping theorem that
    
\begin{align*}
    & A_{nj} \overset{a.s.}{\rightarrow} \sum_{r=1}^{k^*}\frac{|I_j \cap I_r^*|}{|I_j|}{\sigma_r^*}^2 \quad;\\
    & B_{nj} \overset{a.s.}{\rightarrow} 0 \quad; \\
    & C_{nj} \overset{a.s.}{\rightarrow} \sum_{r=1}^{k^*}\frac{|I_j \cap I_r^*|}{|I_j|} (\mu_r^* - \mu_j)^2 \quad. \\
\end{align*}
   
Hence

\begin{equation*}
    \hat{\sigma}_j^2 \overset{a.s.}{\longrightarrow} \sum_{r=1}^{k^*}\frac{|I_j \cap I_r^*|}{|I_j|}{\sigma_r^*}^2 + \sum_{r=1}^{k^*}\frac{|I_j \cap I_r^*|}{|I_j|} (\mu_r^* - \mu_j)^2 =: \sigma_j^2 \quad.
\end{equation*}

Since the estimators converge for all blocks, the empirical log-likelihood limit is then

\begin{equation*}
    \frac{1}{n}l(C; \mathbf{X}) \overset{a.s.}{\longrightarrow} -\frac{m}{2}(\log(2\pi)+1)-\frac{1}{2}\sum_{j=1}^{k}|I_j|\log(\sigma_j^2) =: l^*(C) \quad.
\end{equation*}

We now proceed to verify that the hypothesis hold.

\begin{itemize}
    \item[(i)]  Take any subset $C$ such that $C^* \not \subseteq C$. First, notice we can rewrite
    
\begin{equation*}
    \sigma_j^2 = \sum_{r=1}^{k^*}\frac{|I_j \cap I_r^*|}{|I_j|} ({\sigma_r^*}^2 + (\mu_r^* - \mu_j)^2) \quad.
\end{equation*}
    
    Since $-\log$ is strictly convex, we have
    
\begin{align*}
    -\frac{1}{2}\sum_{j=1}^{k}|I_j|\log(\sigma_j^2)
    & < -\frac{1}{2}\sum_{j=1}^{k}|I_j|\sum_{r=1}^{k^*}\frac{|I_j \cap I_r^*|}{|I_j|}\log({\sigma_r^*}^2 + (\mu_r^* - \mu_j)^2) \quad.
\end{align*}

Notice

\begin{align*}
    -\frac{1}{2}\sum_{j=1}^{k}|I_j|\sum_{r=1}^{k^*}\frac{|I_j \cap I_r^*|}{|I_j|}\log({\sigma_r^*}^2 + (\mu_r^* - \mu_j)^2) &= -\frac{1}{2}\sum_{r=1}^{k^*}\sum_{j=1}^{k}|I_j \cap I_r^*|\log({\sigma_r^*}^2 + (\mu_r^* - \mu_j)^2)\\
    &\leq -\frac{1}{2}\sum_{r=1}^{k^*}|I_r^*|\log({\sigma_r^*}^2) \quad,
\end{align*}
    
    and therefore
    
\begin{align*}
    l^*(C)  
    &= -\frac{m}{2}(\log(2\pi)+1)-\frac{1}{2}\sum_{j=1}^{k}|I_j|\log(\sigma_j^2)\\
    &< -\frac{m}{2}(\log(2\pi)+1)-\frac{1}{2}\sum_{r=1}^{k^*}|I_r^*|\log({\sigma_r^*}^2)\\
    &= l^*(C^*)\quad,
\end{align*}
 
    which finishes the proof for $\textbf{(i)}$.
   
   %%% Proof (ii)
    \item[(ii)] Consider any set $C$ such that $C^* \subseteq C$. Define $\mathcal{I}_r(C) = \{ j\,\in\, (1:{k}) | I_j \subseteq I_r^* \}$, the set of all indices whose blocks defined by $C$ are contained in $I_r^*$. If $C$ does not segment $I_r^*$, then there is only one index in $\mathcal{I}_r$ and the set that it indexes is exactly $I_r^*$. 
    
    The log-likelihood difference is
    
\begin{align*}
    l(C; \mathbf{X}) - l(C^*;\mathbf{X})
    &=  \frac{n}{2} \sum_{r=1}^{k^*}|I_r^*|\left( \log({\hat{\sigma}_r}^2) - \sum_{j\,\in\, \mathcal{I}_r(C)}\frac{|I_j|}{|I_r^*|}\log({\hat{\sigma}_j}^2) \right)\\
    &= \frac{1}{2} \sum_{r=1}^{k^*}\left(\sum_{j\,\in\, \mathcal{I}_r(C)}n|I_j|\log\left(\frac{{\hat{\sigma}_r}^2}{{\hat{\sigma}_j}^2}\right) \right) \quad.
\end{align*}
    
    When there is no splitting on $I_r^*$ by $C$, the $r$-th term is zero. Lets concentrate on the non zero terms. Using the inequality $\log(x) \leq x - 1 \quad, \forall \, x > 0$, it follows that
    
\begin{align*}
    \sum_{ j\,\in\, \mathcal{I}_r(C) }n|I_j|\log\left(\frac{{\hat{\sigma}_r}^2}{{\hat{\sigma}_j}^2}\right)
    & \leq \sum_{j\,\in\, \mathcal{I}_r(C) }n|I_j|\left(\frac{{\hat{\sigma}_r}^2 - {\hat{\sigma}_j}^2}{{\hat{\sigma}_j}^2}\right)
\end{align*}
    
    The empirical variance estimator for the whole block satisfies
    
\begin{align*}
    {\hat{\sigma}_r}^2 
    &= \frac{1}{n|I_r|} \sum_{c \,\in\, I_r^*}\sum_{i=1}^n (X_c^{(i)} - \hat{\mu}_r)^2 \\
    &= \frac{1}{n|I_r|} \sum_{c \,\in\, I_r^*}\sum_{i=1}^n \left[\left(X_c^{(i)} - \mu_r^*\right)^2\right] - (\hat{\mu}_r - \mu_r^*)^2 \\
    &\leq \frac{1}{n|I_r|} \sum_{c \,\in\, I_r^*}\sum_{i=1}^n \left[\left(X_c^{(i)} - \mu_r^*\right)^2\right] \quad.\\
\end{align*}
    
    A similar calculation for the variance of the nested blocks yields
 
 \begin{align*}
    {\hat{\sigma}_j}^2 
    &= \frac{1}{n|I_j|} \sum_{c \,\in\, I_j}\sum_{i=1}^n (X_c^{(i)} - \hat{\mu}_j)^2 \\
    &= \frac{1}{n|I_j|} \sum_{c \,\in\, I_j}\sum_{i=1}^n \left[\left(X_c^{(i)} - \mu_r^*\right)^2\right] - (\hat{\mu}_j - \mu_r^*)^2 \\
\end{align*}  
    
    Defining $\delta_r^2 = \underset{\mathcal{I}_r(C)}{\min}\hat{\sigma}_j^2$, and $j' = \underset{\mathcal{I}_r(C)}{\argmax} (\hat{\mu}_j - \mu_r^*)^2$, we have
    
\begin{align*}
    \sum_{j\,\in\, \mathcal{I}_r(C) }n|I_j|\left(\frac{{\hat{\sigma}_r}^2 - {\hat{\sigma}_j}^2}{{\hat{\sigma}_j}^2}\right)
    &\leq \frac{n}{\delta_r^2}\sum_{j\,\in\, \mathcal{I}_r(C) }|I_j|\left({\hat{\sigma}_r}^2 - {\hat{\sigma}_j}^2\right)\\
    &= \frac{n}{\delta_r^2}\left(|I_r^*|\hat{\sigma}_r^2 - \sum_{j\,\in\, \mathcal{I}_r(C) } |I_j|\hat{\sigma}_j^2 \right)\\
    &\leq \frac{n}{\delta_r^2}\left( \sum_{j\,\in\, \mathcal{I}_r(C)} (\hat{\mu}_j - \mu_r^*)^2 \right)\\
    &\leq \frac{|I_r^*|n}{\delta_r^2}(\hat{\mu}_{j'} - \mu_r^*)^2\\
    &= \frac{|I_r^*|}{|I_{j'}|^2\delta_r^2}\left[\frac{1}{\sqrt{n}} \sum_{c \,\in\, I_{j'}}\sum_{i=1}^n \left(X_c^{(i)} - \mu_r^*\right) \right]^2
\end{align*}
    
    Define
    
\begin{equation*}
    S_{j^*} = \left[\frac{1}{\sqrt{n\log\log n}} \sum_{c \,\in\, I_{j'}}\sum_{i=1}^n \left(X_c^{(i)} - \mu_r^*\right)\right] 
\end{equation*}
    
    By the law of the iterated logarithm, there exists $\epsilon_{j^*} > 1$ such that
    
\begin{equation*}
    \underset{n \rightarrow \infty}{\limsup}\, S_{j^*} < \epsilon_{j^*} \quad.
\end{equation*}
    
    By $\limsup$ properties,

\begin{equation*}
    \underset{n \rightarrow \infty}{\limsup}\, S_{j^*}^2 < \epsilon_{j^*}^2 \quad.
\end{equation*}

    Notice that $\delta_r^2 \overset{a.s.}{\rightarrow} {\sigma_r^*}^2$, hence $\underset{n\rightarrow\infty}{\limsup}\,\delta_r^2 = {\sigma_r^*}^2$. 
    Dividing the terms inside each block by $\log\log n$, we have
    
\begin{align*}
    \underset{n\rightarrow\infty}{\limsup}\,\frac{n|I_j|}{\log\log n}\sum_{j\,\in\, \mathcal{I}_r(C) }\left(\frac{{\hat{\sigma}_r}^2 - {\hat{\sigma}_j}^2}{{\hat{\sigma}_j}^2}\right)
    &\leq \underset{n\rightarrow\infty}{\limsup}\, \frac{|I_r^*|}{|I_{j^*}|^2\delta_r^2}S_{j^*}^2\\
    &\leq \frac{|I_r^*|}{|I_{j^*}|^2}  \underset{n\rightarrow\infty}{\limsup}\,\left( \frac{1}{\delta_r^2}\right)\underset{n\rightarrow\infty}{\limsup}\,\left(S_{j^*}^2\right)\\
    &\leq \frac{|I_r^*|}{|I_{j^*}|^2}\frac{1}{{\sigma_r^*}^2}\epsilon_j^2\quad.
\end{align*}

    Finally
    
\begin{align*}
    \frac{1}{\log\log n}l(C; \mathbf{X}) - l(C^*;\mathbf{X})
    &\leq \underset{n\rightarrow\infty}{\limsup}\, \frac{1}{\log\log n}l(C; \mathbf{X}) - l(C^*;\mathbf{X}) \\
    &\leq \sum_{r=1}^{k^*} \underset{n\rightarrow\infty}{\limsup} \,\frac{n|I_j|}{\log\log n}\sum_{j\,\in\, \mathcal{I}_r(C) }\left(\frac{{\hat{\sigma}_r}^2 - {\hat{\sigma}_j}^2}{{\hat{\sigma}_j}^2}\right)\\
    &\leq \sum_{r=1}^{k^*}\frac{|I_r^*|}{|I_{j^*}|^2}\frac{1}{{\sigma_r^*}^2}\epsilon_j^2\\
    &\leq \epsilon \quad,
\end{align*}

    for some $\epsilon > 0$. This establishes conditions $(ii)$, and therefore the PL estimator for this family is consistent.

\end{itemize}
